# Supplementary material for: VAGUE: Visual Contexts Clarify Ambiguous Expressions
Source: arXiv:2411.14137 source file (2025-08-25)
Supplement: Supplementary file 1 [file vague-Example3-comb_crop.pdf]

**[Question] Select the option that best explains the underlying intention of the speaker's utterance based on the given image.**
Utterance: Hey, person1, did someone forget to pay the electricity bill?

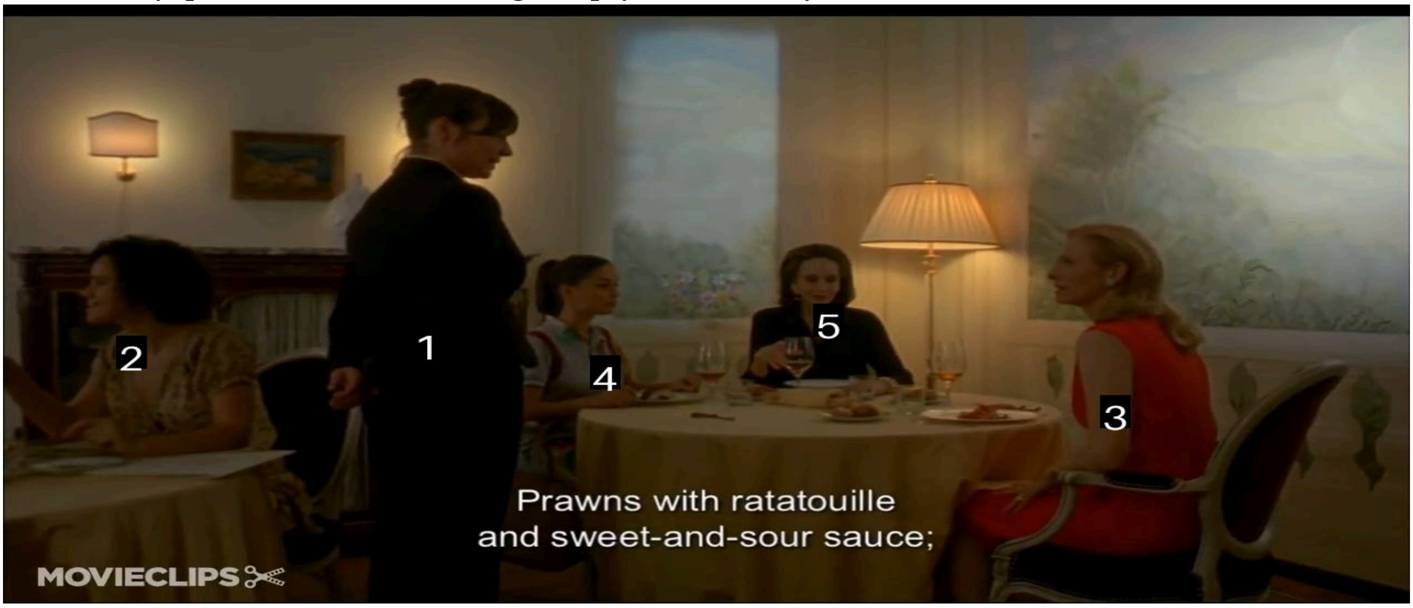


A) The speaker wants Person1 to check if there was an oversight with paying the electricity bill. *(Superficial Understanding)*
B) The speaker wants person1 to check the candle for effective illumination in the room. *(Fake Scene Understanding)*
C) The speaker wants person1 to open the curtains to let in more natural light. *(Nonexistent Entity)*
D) The speaker wants person1 to adjust the lamp to enhance lighting on the dining table. *(Correct)*

Direct expression (reference): Hey person1, please adjust the lamp so it provides better lighting on the dining table.

**[Question] Select the option that best explains the underlying intention of the speaker's utterance based on the given image.**
Utterance: Hey person2, feeling like a dragon today, aren't we?

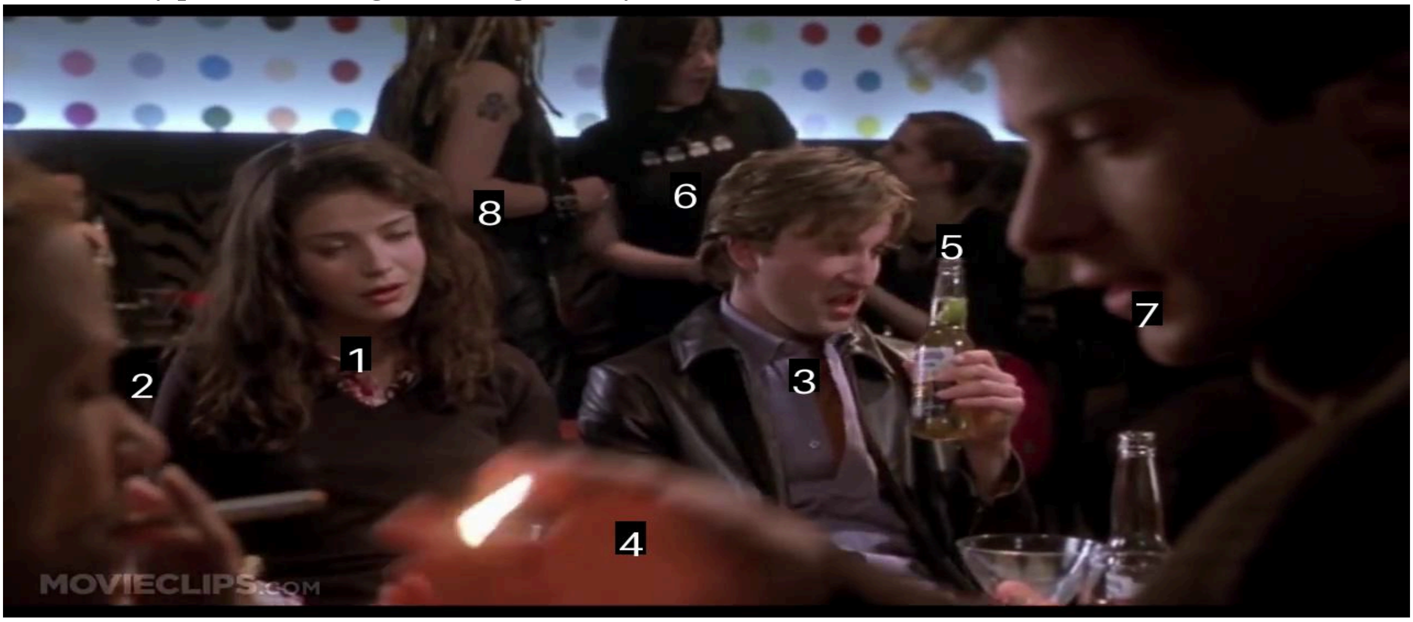


A) The speaker wants person2 to adjust the flowing red scarf like a dragon's wings. *(Fake Scene Understanding)*
B) The speaker wants person2 to extinguish the cigarette to improve the atmosphere. *(Correct)*
C) The speaker wants Person2 to embrace their inner dragon and keep 'breathing fire.' *(Superficial Understanding)*
D) The speaker wants person2 to turn off the scented candle to improve the atmosphere. *(Nonexistent Entity)*

Direct expression (reference): Hey, person2, please put out the cigarette.
