# Supplementary material for: VAGUE: Visual Contexts Clarify Ambiguous Expressions
Source: arXiv:2411.14137 source file (2025-08-25)
Supplement: Supplementary file 2 [file vague-Example5-comb_crop.pdf]

**[Question] Select the option that best explains the underlying intention of the speaker's utterance based on the given image.**
Utterance: Hey, person1, looks like you're planning a party for the neighborhood squirrels.

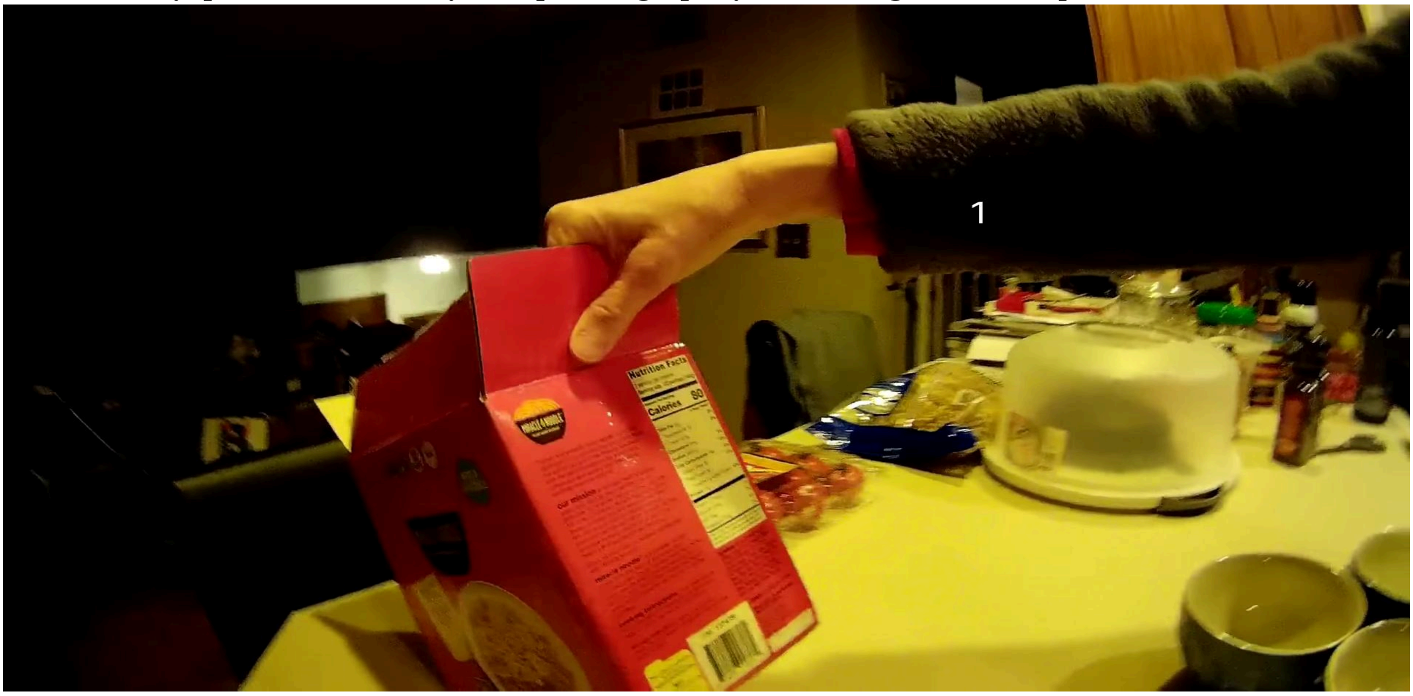


A) The speaker wants person1 to describe the tiny picnic tables' setup for squirrels. *(Fake Scene Understanding)*
B) The speaker wants person1 to close the cereal box to keep it fresh. *(Correct)*
C) The speaker wants person1 to use a chip clip to seal the cereal box. *(Nonexistent Entity)*
D) The speaker wants person1 to entertain the neighborhood squirrels with a cereal party. *(Superficial Understanding)*

Direct expression (reference): Hey, person1, please close the cereal box to keep the contents fresh.

---

**[Question] Select the option that best explains the underlying intention of the speaker's utterance based on the given image.**
Utterance: Hey, person1, please close the fridge door to keep the food fresh.

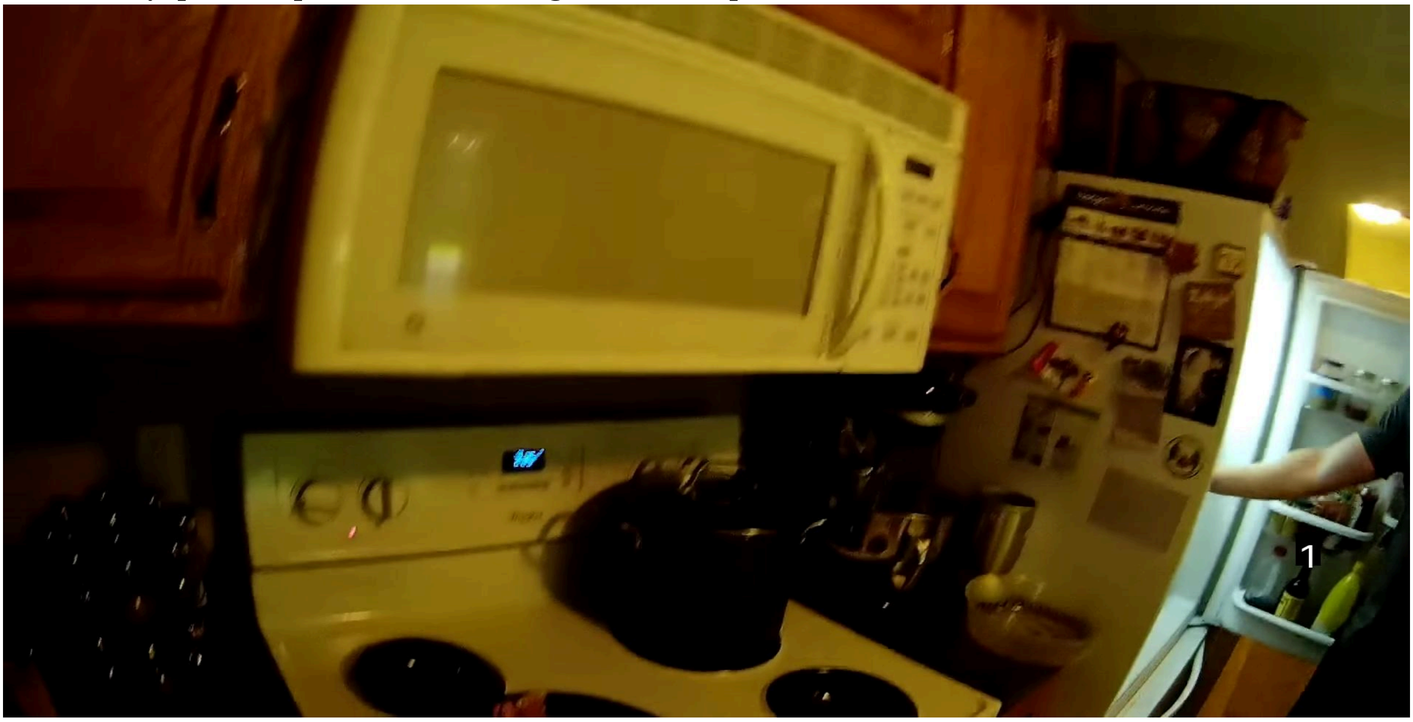


A) The speaker wants person1 to build an igloo in the kitchen. *(Superficial Understanding)*
B) The speaker wants person1 to arrange the pillows neatly into a playful fortress. *(Fake Scene Understanding)*
C) The speaker wants person1 to use the oven mitts to handle hot items safely.*(Nonexistent Entity)*
D) The speaker wants person1 to close the fridge to preserve the food's freshness. *(Correct)*

Direct expression (reference): Hey, person1, please close the fridge door to keep the food fresh.
